# Supplementary material for: Emerging Properties in Self-Supervised Vision Transformers
Source: arXiv:2104.14294 source file (2021-05-24)
Supplement: Supplementary file 1 [file supp.tex]

\documentclass[10pt,twocolumn,letterpaper]{article}
\usepackage{iccv}
\usepackage{times}
\usepackage{epsfig}
\usepackage{url}            % simple URL typesetting
\usepackage{graphbox}
\usepackage{booktabs}       % professional-quality tables
\usepackage{amsfonts}       % blackboard math symbols
\usepackage{nicefrac}       % compact symbols for 1/2, etc.
\usepackage{microtype}      % microtypography
\usepackage{comment}
\usepackage{amsmath,amssymb} % define this before the line numbering.
\usepackage{caption}
\usepackage{mathtools}
\usepackage{graphicx}
\usepackage{soul}
\usepackage[subrefformat=parens]{subfig}
\usepackage{enumitem}

\usepackage{xspace}
\usepackage{multirow}
\usepackage{array}
\usepackage{layouts}
\usepackage{algorithm}
\usepackage{bbding}
\usepackage{listings}
\usepackage{pifont}
\usepackage{wasysym}
\usepackage{float}
\usepackage{soul}
\usepackage{dblfloatfix}
\usepackage{footnote}
\makesavenoteenv{tabular}
\makesavenoteenv{table}
\makesavenoteenv{figure}
\usepackage[dvipsnames]{xcolor}

\usepackage{xcolor,colortbl}
\definecolor{Gray}{gray}{0.85}
\newcolumntype{g}{>{\columncolor{Gray}}c}

\usepackage[pagebackref=true,breaklinks=true,letterpaper=true,colorlinks,bookmarks=false]{hyperref}
\usepackage{cleveref}

% \iccvfinalcopy % *** Uncomment this line for the final submission

 % *** Enter the ICCV Paper ID here

\ificcvfinal\pagestyle{empty}\fi

\usepackage{xcolor,colortbl}
\definecolor{Gray}{gray}{0.85}
\definecolor{ffe1da}{RGB}{255,225,218}
\definecolor{F7E0D5}{RGB}{247,224,213}
\colorlet{Light}{White!0!F7E0D5}
\newcolumntype{g}{>{\columncolor{Light}}c}
\usepackage{pythonhighlight}

\begin{document}

\title{Supplementary Material for \\
Self-Supervised Learning of Visual Transformers with a Momentum Teacher}
\author{First Author\\
Institution1\\
Institution1 address\\
{\tt\small firstauthor@i1.org}
\and
Second Author\\
Institution2\\
First line of institution2 address\\
{\tt\small secondauthor@i2.org}
}

\maketitle
% Remove page # from the first page of camera-ready.
\ificcvfinal\thispagestyle{empty}\fi

% textwidth: \printinunitsof{in}\prntlen{\textwidth}
% linewidth: \printinunitsof{in}\prntlen{\linewidth}

\input{appendix.tex}

\clearpage

{\small
\bibliographystyle{ieee_fullname}
\bibliography{egbib}
}

\end{document}
